# Supplementary material for: Path Integral Molecular Dynamics for Bosons
Source: arXiv:1905.09053 ancillary file (2019-05-22)
Supplement: Supplementary file 1 [file SI.pdf]

# Supporting Information: Path-integral Molecular Dynamics for Bosons

Barak Hirshberg and Valerio Rizzi

*Department of Chemistry and Applied Biosciences,*

*ETH Zurich, 8092 Zurich, Switzerland and*

*Institute of Computational Sciences, Università della Svizzera italiana,*

*via G. Buffi 13, 6900 Lugano, Switzerland*

Michele Parrinello

*Department of Chemistry and Applied Biosciences,*

*ETH Zurich, 8092 Zurich, Switzerland*

*Institute of Computational Sciences, Università della Svizzera italiana,*

*via G. Buffi 13, 6900 Lugano, Switzerland and*

*Italian Institute of Technology, Via Morego 30, 16163 Genova, Italy*

(Dated: May 22, 2019)

## CALCULATING THE FORCES

To perform PIMD simulations for Bosons, one needs to evaluate the force acting on each bead of each particle, due to the potential $V_B^{(N)}$. Similarly to the potential, the force can be written as a recurrence relation, allowing to evaluate it without enumerating all the unique ring-polymer diagrams. We start by taking the logarithm of the recurrence relation from the main text

$$V_B^{(N)}(R_1, ..., R_N) = -\frac{1}{\beta} \ln \left[ \frac{1}{N} \sum_{k=1}^{N} e^{-\beta\left(E_N^{(k)} + V_B^{(N-k)}\right)}, \right]. \tag{1}$$

defining $E_N^{(k)}(R_{N-k+1}, ..., R_N)$ as in the main text. The force acting on bead $j$ of particle $l$ is

$$-\nabla_{\boldsymbol{r}_l^j} V_B^{(N)}(R_1, ..., R_N) = -\frac{\sum_{k=1}^{N} \left[ \nabla_{\boldsymbol{r}_l^j} E_N^{(k)} + \nabla_{\boldsymbol{r}_l^j} V_B^{(N-k)} \right] e^{-\beta\left(E_N^{(k)} + V_B^{(N-k)}\right)}}{\sum_{k=1}^{N} e^{-\beta\left(E_N^{(k)} + V_B^{(N-k)}\right)}}, \tag{2}$$

where $\nabla_{\boldsymbol{r}_l^j} V_B^{(0)} = 0$ and $V_B^{(0)} = 0$. If $l$ belongs to $(N-k+1, ..., N)$, the derivative of $E_N^{(k)}(R_{N-k+1}, ..., R_N)$ is given by

$$\nabla_{\boldsymbol{r}_l^j} E_N^{(k)}(R_{N-k+1}, ..., R_N) = m\omega_P^2 (2\boldsymbol{r}_l^j - \boldsymbol{r}_l^{j+1} - \boldsymbol{r}_l^{j-1}). \tag{3}$$

If not, $\nabla_{\boldsymbol{r}_l^j} E_N^{(k)}(R_{N-k+1}, ..., R_N) = 0$. In Equation 3, $\boldsymbol{r}_N^{P+1} = \boldsymbol{r}_1^1$ and $\boldsymbol{r}_l^{P+1} = \boldsymbol{r}_{l+1}^1$ otherwise. In addition, $\boldsymbol{r}_1^0 = \boldsymbol{r}_N^P$ and $\boldsymbol{r}_l^0 = \boldsymbol{r}_{l-1}^P$ otherwise.

## ESTIMATOR FOR THE TOTAL ENERGY

The estimator for the total energy, presented also in the main text, is given by

$$\langle E \rangle = \frac{PdN}{2\beta} + \langle U \rangle + \left\langle V_B^{(N)} + \beta \frac{\partial V_B^{(N)}}{\partial \beta} \right\rangle. \tag{4}$$

where $V_B^{(N)} + \beta \frac{\partial V_B^{(N)}}{\partial \beta}$ is also evaluated using a recurrence relation

$$V_B^{(N)} + \beta \frac{\partial V_B^{(N)}}{\partial \beta} = \frac{\sum_{k=1}^{N} \left[ V_B^{(N-k)} + \beta \frac{\partial V_B^{(N-k)}}{\partial \beta} - E_N^{(k)} \right] e^{-\beta\left(E_N^{(k)} + V_B^{(N-k)}\right)}}{\sum_{k=1}^{N} e^{-\beta\left(E_N^{(k)} + V_B^{(N-k)}\right)}}, \tag{5}$$

and $V_B^{(0)} + \beta \frac{\partial V_B^{(0)}}{\partial \beta} = 0$. For $N = 1$, Equation 4 reduces to the usual thermodynamic estimator for the total energy of a single particle.

## COST OF EVALUATING THE RECURRENCE RELATIONS

The most important part in performing PIMD simulations for Bosons is the evaluation of the forces acting on all beads of all particles. However, using the recurrence relation in Equation 2 requires the evaluation of $V_B^{(1)}, ..., V_B^{(N)}$ first. In order to evaluate the potential for a given $N$, one must loop over $m = (1, ..., N)$ and, for every $m$, evaluate $E_N^{(k)}(R_{N-k+1}, ..., R_N)$ for $k = (1, ..., m)$. The cost of evaluating $E_N^{(k)}(R_{N-k+1}, ..., R_N)$ scales linearly with $kP$. Therefore, the computational scaling of evaluating $V_B^{(1)}, ..., V_B^{(N)}$ can be estimated as

$$\sum_{m=1}^{N} \sum_{k=1}^{m} kP = P \sum_{m=1}^{N} \sum_{k=1}^{m} k = P \sum_{m=1}^{N} \frac{m(m+1)}{2} \sim \mathcal{O}(PN^3) \tag{6}$$

Then, the force acting on bead $j$ of particle $l$ is obtained using a similar procedure: for a given $N$, one must loop over $m = (1, ..., N)$ and, for every $m$, evaluate $\nabla_{\boldsymbol{r}_l^j} E_N^{(k)}(R_{N-k+1}, ..., R_N)$ for $k = (1, ..., m)$. However, the cost of evaluating $\nabla_{\boldsymbol{r}_l^j} E_N^{(k)}$ is independent of $k$. Therefore, the computational scaling of evaluating $\nabla_{\boldsymbol{r}_l^j} V_B^{(1)}, ..., \nabla_{\boldsymbol{r}_l^j} V_B^{(N)}$ can be estimated as

$$\sum_{m=1}^{N} \sum_{k=1}^{m} 1 = \sum_{m=1}^{N} m \sim \mathcal{O}(N^2) \tag{7}$$

Finally, the cost of evaluating all $PN$ forces required leads to a scaling of $\mathcal{O}(PN^3)$. A numerical confirmation of this analysis is provided in Figure 1. To isolate the scaling of the algorithm presented in this paper we first tested the scaling on a C++ implementation outside of LAMMPS and obtained a slope of $\sim 3$ on a log-log scale. We then verified that similar scaling is obtained for the LAMMPS implementation by measuring the average time required per MD step (taken over 1000 steps) for different $N$. The slope on log-log scale for this implementation is $\sim 2.5$.

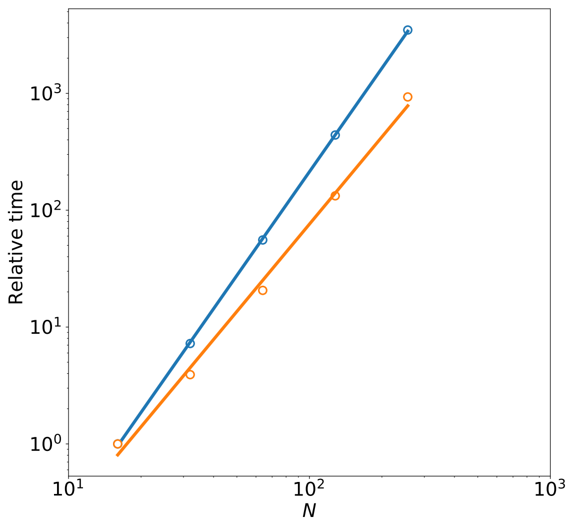


FIG. 1. Blue circles show relative time for evaluation of the forces acting on all particles as a function of the number of particles $N$. The results are calculated using a designated C++ implementation using randomly sampled numbers representing the coordinates of each bead of each particle. Orange circles show the relative time per LAMMPS MD step as a function of the number of particles $N$. The results are averages accumulated over 1000 time steps. The lines are linear fits to the numerical results on log-log scale.

## NUMBER OF ENERGY TERMS

Figure 2 shows the number of terms needed when calculating all permutations (blue circles), just the unique diagrams (orange squares) and the number of energy terms when evaluating $V_B^{(N)}$ (green triangles). It can be seen that for $N < 12$, the number of unique diagrams is actually smaller than the number of terms required for the evaluation of $V_B^{(N)}$. However, for larger $N$ the number of unique diagrams grows exponentially.

## NUMERICAL DETAILS

The numerical evaluation of the recurrence relations presented in this Letter require some care, since they involve summation over $N$ of terms of the form $e^{-\beta E_N^{(k)}}$. Since $E_N^{(k)} \geq 0$ and grows with $k$, these terms can become exponentially small. Therefore, we evaluate the potential using

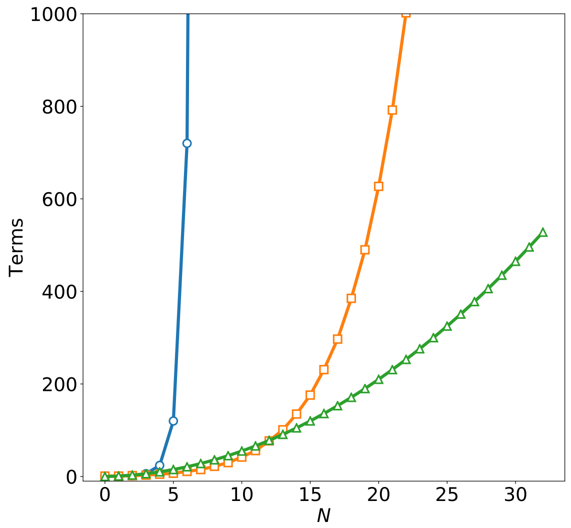


FIG. 2. The number of terms which are evaluated as a function of $N$, the number of particles. Blue circles represent enumerating all permutations and is equal to $N!$. Orange squares represent enumerating just the unique diagrams and is equal to the number of partitions of integer $N$, which scales exponentially with $N$. Green triangles represent the binomial coefficient $b(N) = N(N+1)/2$, which represent the number of energy evaluations required to calculate the potential $V_B^{(N)}$. Lines between points were added for clarity.

$$V_B^{(N)}(R_1, ..., R_N) = \tilde{E} - \frac{1}{\beta} \ln \left[ \frac{1}{n} \sum_{k=1}^{N} e^{-\beta \left( E_N^{(k)} + V_B^{(N-k)} - \tilde{E} \right)} \right]. \quad (8)$$

The results are independent of the choice of $\tilde{E}$, but we can choose it in order to obtain improved numerical stability. We find that in most cases choosing the energy of the longest ring-polymer $E_N^{(N)}$ was efficient. In other cases, the average between $E_N^{(N)}$ and $V_B^{(N-1)}$ was used. Similar equations were used for the forces.

## CONVERGENCE WITH RESPECT TO $P$

Figures 3, 4 and 5 present the convergence of the total energy with respect to the number of beads, $P$. For non-interacting particles, the results are converged for $P = 36$. For calculations using $N = 2-4$ and all range of interaction strengths we used $P = 72$. This value was determined from convergence plots for $N = 4$ and $g = 16$, which were slowest to

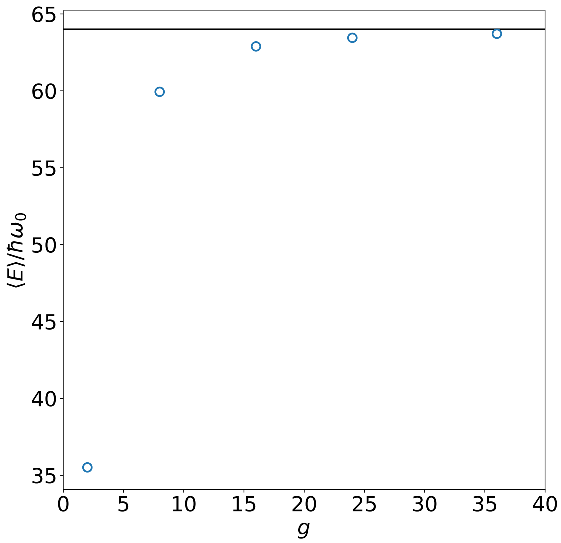


FIG. 3. Convergence of the total energy for $N = 64$ non-interacting particles as a function of the number of beads, $P$. The black line represents the ground-state energy of 64 non-interacting Bosons in the 2D trap. The calculations were performed at a temperature corresponding to $\beta\hbar\omega_0 = 6$.

converge. For $N = 32$ interacting particles, at the range of interactions studied ($g = 0 - 3$), the results were converged (to within $\sim 2\%$) already for $P = 36$, which was used in all simulations.

## RESULTS FOR NON-INTERACTING PARTICLES

The results obtained for $N = 2, 3, 4, 32$ and 64 non-interacting particles for $\beta\hbar\omega_0 = 6$ are shown in Figure 6. The calculations were performed using $P = 36$ beads and agree to within $\sim 0.5\%$ with the analytical ground-state energies. The ground-state energy is identical for both distinguishable particles and Bosons. Therefore, we also calculated the temperature dependence for the average energy for a system of $N = 2$ and 16 particles and show that we obtain not only the correct ground-state energy but also the correct statistics. The results are presented in Figure 7. It can be seen that at $\beta\hbar\omega_0 = 6$ the energy is already very close to the $T = 0$ ground-state value.

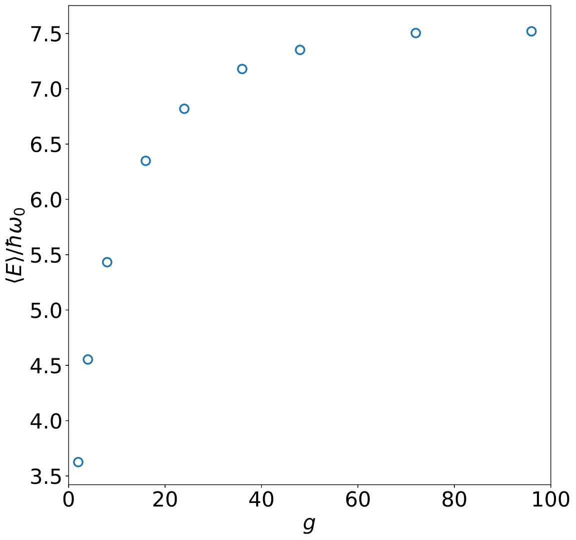


FIG. 4. Convergence of the total energy for $N = 4$ particles as a function of the number of beads, $P$. Blue circles represent values of $g = 16$. The calculations were performed at a temperature corresponding to $\beta\hbar\omega_0 = 6$.

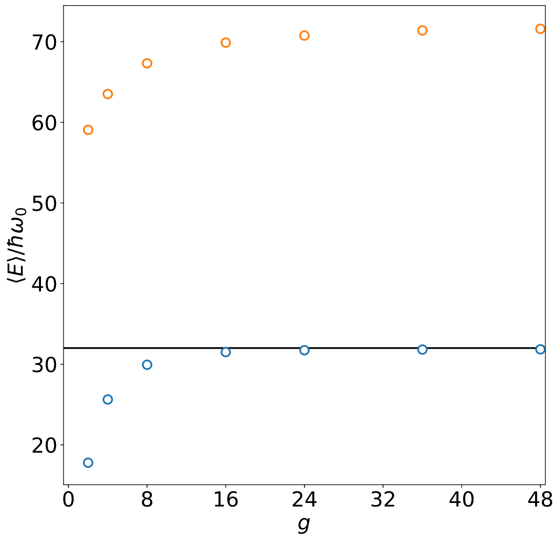


FIG. 5. Convergence of the total energy for $N = 32$ particles as a function of the number of beads, $P$. Blue and orange circles represent values of $g = 0$ and $g = 1$, respectively. The results for $g = 3$ are not shown but were converged to within $\sim 2\%$ for $P = 36$. The black line represents the ground-state energy of 32 non-interacting Bosons in the 2D trap. The calculations were performed at a temperature corresponding to $\beta\hbar\omega_0 = 6$.

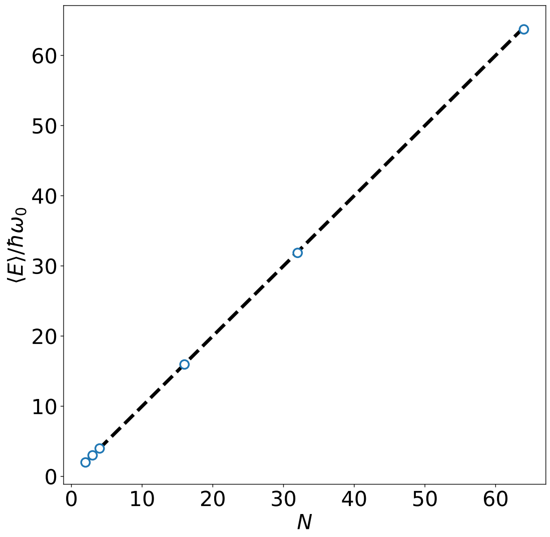


FIG. 6. The total energy for non-interacting particles as a function of the number of particles, $N$. The black line represents the exact result for the ground-state energy. The calculations were performed at a temperature corresponding to $\beta\hbar\omega_0 = 6$.

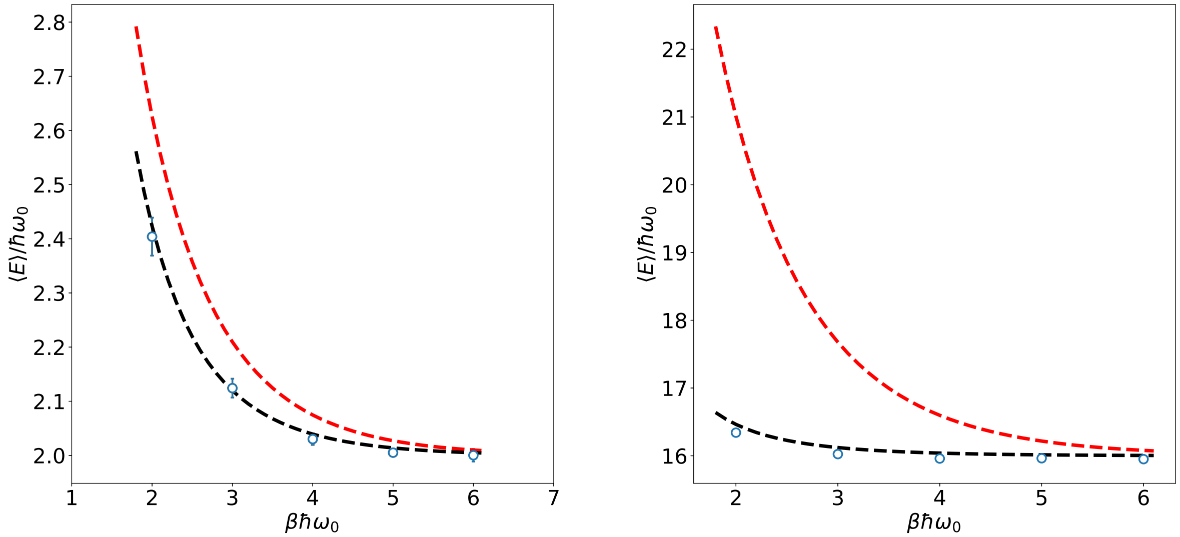


FIG. 7. The average total energy for $N = 2$ (left) and 16 non-interacting particles as a function of inverse temperature. The red and black lines represent the exact results for distinguishable particles and Bosons, respectively. Maximal absolute deviation is $\sim 0.7\%$.
